# Supplementary material for: Diffusions on a space of interval partitions: construction from marked L\'evy processes
Source: arXiv:1909.02584 ancillary file (2019-09-05)
Supplement: Supplementary file 1 [file IPP1_diff_supplement_23Aug2019_MW.pdf]

**DIFFUSIONS ON A SPACE OF INTERVAL PARTITIONS:  
CONSTRUCTION FROM MARKED LÉVY PROCESSES.  
SUPPLEMENT A: MEASURE THEORETIC DETAILS\***

BY NOAH FORMAN<sup>†</sup>, SOUMIK PAL<sup>‡</sup>, DOUGLAS RIZZOLO<sup>§</sup>,  
AND MATTHIAS WINKEL<sup>¶</sup>

*McMaster University<sup>†</sup>, University of Washington<sup>‡</sup>,  
University of Delaware<sup>§</sup>, University of Oxford<sup>¶</sup>*

**1. Overview.** This supplement contains some technical details of notions and results that we use in the main paper. Specifically, the structure of this supplement is, as follows. In Section 2 we formalise the notion of disintegration and an existence result in the context of a scaling operation. In Section 3 we discuss random counting measures and establish that various counting measures are boundedly finite. In Section 4 we show the measurability of the skewer map, cutoff functions and associated point measures of clades, and we prove some related technical results.

**2. Scaling and disintegration.** In Section 2.1.A of the main paper we briefly discussed disintegration and scaling. Here is a formal definition and a fuller discussion of the relevant notions.

DEFINITION 1 (Pushforward and disintegration). Let  $(\mathcal{S}, \Sigma(\mathcal{S}), \mu)$  be a  $\sigma$ -finite measure space and  $\phi: \mathcal{S} \rightarrow \mathcal{T}$  a measurable function into a measurable space  $(\mathcal{T}, \Sigma(\mathcal{T}))$ . We use notation  $\mu(\phi \in B) := \phi_*\mu(B) := \mu(\phi^{-1}(B))$ ,  $B \in \Sigma(\mathcal{T})$ , for the *pushforward* of  $\mu$  under  $\phi$ . A  $\phi$ -*disintegration* of  $\mu$  is a map  $y \mapsto \mu_y$  from  $\mathcal{T}$  to probability measures on  $(\mathcal{S}, \Sigma(\mathcal{S}))$  with the following properties.

- (i) For each  $A \in \Sigma(\mathcal{S})$  fixed, the map  $y \mapsto \mu_y(A)$  is  $\Sigma(\mathcal{T})$ -measurable.
- (ii) For each  $y \in \mathcal{T}$ , we have  $\mu_y\{x \in \mathcal{S}: \phi(x) \neq y\} = 0$ .
- (iii) Writing  $\nu = \phi_*\mu$ , we have

$$\mu(A) = \int \mu_y(A) d\nu(y) \quad \text{for every } A \in \Sigma(\mathcal{S}).$$

---

\*This research is partially supported by NSF grants DMS-1204840, DMS-1308340, DMS-1612483, DMS-1855568, UW-RRF grant A112251, EPSRC grant EP/K029797/1

This is narrower in several respects than the most general definition of a disintegration. In general, disintegrations are not required to give probability kernels. For an excellent, broader treatment, see [3].

In the setting of excursion theory, it is a standard technique to view a  $\sigma$ -finite excursion measure as a product between a  $\sigma$ -finite measure on  $(0, \infty)$  and a probability distribution on the space of normalized excursions. This is possible when the excursion measure has an invariance property relative to some scaling map. This product decomposition is equivalent to a unique disintegration: to each  $a > 0$  we associate a probability distribution on excursions of length  $a$ , by scaling the random normalized excursion by a factor of  $a$ . See [4] for work related to this method in the setting of stable Lévy processes. Williams' decomposition of Brownian excursion fits into this framework, with excursions normalized by amplitude rather than length; see [9, Theorem 22.15] or [10, Theorems XII.4.2 and XII.4.5].

Here is a more general statement of this principle that scaling maps give rise to unique disintegrations. We leave its proof to the reader.

**LEMMA 2 (Scaling and disintegration).** *Let  $(\mathcal{S}, \Sigma(\mathcal{S}), \mu)$  be a  $\sigma$ -finite measure space and  $\theta: \mathcal{S} \rightarrow (0, \infty)$  a measurable function. Suppose  $\odot: (0, \infty) \times \mathcal{S} \rightarrow \mathcal{S}$  is a measurable scaling map in the sense that there exists some  $p > 0$  such that, for every  $b, c > 0$ ,  $x \in \mathcal{S}$ , and  $A \in \Sigma(\mathcal{S})$ ,*

$$b \odot (c \odot x) = bc \odot x, \quad 1 \odot x = x, \quad \text{and} \quad \mu(c \odot A) = c^{-p} \mu(A).$$

*Suppose further that there exists some  $q > 0$  such that for every  $c > 0$  and  $x \in \mathcal{S}$ ,*

$$\theta(c \odot x) = c^q \theta(x) \quad \text{and} \quad \mu\{x \in \mathcal{S}: \theta(x) > 1\} < \infty.$$

*Then there exists a  $\theta$ -disintegration of  $\mu$ , which we denote by  $a \mapsto \mu_a$ , unique with the property that for every  $a > 0$ , if  $X$  has law  $\mu_a$  then  $a^{-1/q} \odot X$  has law  $\mu_1$ . Moreover, for each  $b > 0$ , the measure  $\mu_1$  equals the pushforward of  $\mu(\cdot | \theta(x) > b)$  under the map  $x \mapsto \theta(x)^{-1/q} \odot x$ .*

In the context of Lemma 2, we write  $\mu(\cdot | \theta = a)$  to denote the measure called  $\mu_a$  in the statement of the lemma. In the main paper, we apply this result to several  $\sigma$ -finite (intensity) measures to disintegrate along certain one-dimensional statistics such as excursion length and more general measurable functions such as the scaffolding map  $\xi$  that associates with suitable point measures  $N$  a path  $g = \xi(N)$  in Skorokhod space.

**3. Boundedly finite counting measures.** As indicated in Section 2.1.B, our main reference for random counting measures is [5, 6]. To rigorously apply their results, we need to check that some of our counting

measures are boundedly finite in suitable metric spaces. We also include here some measurability results we need. We begin in the context of excursion theory. In Lemma 2.7 we describe the Pitman–Yor excursion measure  $\Lambda$  of BESQ( $-2\alpha$ ).

**PROPOSITION 3.** *We define a metric  $d_{\mathcal{D}}^A$  on  $\mathcal{E}$  via  $d_{\mathcal{D}}^A(f, g) := d_{\mathcal{D}}(f, g) + |A(f)^{-1} - A(g)^{-1}|$ , where  $d_{\mathcal{D}}$  is the Skorokhod metric and  $A$  the amplitude defined in (2.13). This metric is topologically equivalent to  $d_{\mathcal{D}}$  on  $\mathcal{E}$ . Moreover,  $(\mathcal{E}, d_{\mathcal{D}}^A)$  is separable and complete and  $\Lambda$  is boundedly finite under this metric, i.e.  $\Lambda(B) < \infty$  for all measurable  $B \subset \mathcal{E}$  that are bounded in  $(\mathcal{E}, d_{\mathcal{D}}^A)$ .*

**PROOF.** Note that  $\mathcal{E} \cup \{0\}$  is complete under  $d_{\mathcal{D}}$  and  $1/A$  is continuous under  $d_{\mathcal{D}}$  on  $\mathcal{E}$ . Hence, a  $d_{\mathcal{D}}$ -Cauchy sequence in  $\mathcal{E}$  with non-zero limit converges to the same limit in  $d_{\mathcal{D}}^A$ , and a sequence converging to 0 under  $d_{\mathcal{D}}$  cannot be Cauchy under  $d_{\mathcal{D}}^A$ . This proves the completeness of  $d_{\mathcal{D}}^A$  and its topological equivalence to  $d_{\mathcal{D}}$ . Separability follows from topological equivalence. The reader may confirm that  $\Lambda$  is boundedly finite under  $d_{\mathcal{D}}^A$ .  $\square$

In Definition 2.13, we define various sets of counting measures. The following proposition records some measurability results.

**PROPOSITION 4.** *The  $\sigma$ -algebra  $\Sigma(\mathcal{N}([0, \infty) \times \mathcal{E}))$  on  $\mathcal{N}([0, \infty) \times \mathcal{E})$  generated by the evaluation maps is the Borel  $\sigma$ -algebra of a Polish topology. The sets  $\mathcal{N}^{\text{sp}}$  and  $\mathcal{N}_{\text{fin}}^{\text{sp}}$  are Borel-measurable subsets of  $\mathcal{N}([0, \infty) \times \mathcal{E})$ .*

**PROOF.** By Proposition 3,  $(\mathcal{E}, d_{\mathcal{D}}^A)$  is complete and separable. Thus, the first assertion follows from [5, Theorem A2.6.III]. The measurability of condition (i) in Definition 2.13 follows from the existence of measurable enumerations of points of counting measures; see [6, Proposition 9.1.XII]. Finally, the measurability of conditions (ii) and (iii) in Definition 2.13 follows from the measurability of the evaluation maps  $N \mapsto N(B)$ ,  $B \in \Sigma(\mathcal{N}([0, \infty) \times \mathcal{E}))$ .  $\square$

In (4.3)–(4.4), we define two subsets  $\mathcal{D}_{\text{stb}}$  and  $\mathcal{D}_{\text{exc}}$  of Skorokhod space.

**PROPOSITION 5.**  *$\mathcal{D}_{\text{stb}}$  and  $\mathcal{D}_{\text{exc}}$  are Borel sets in  $(\mathcal{D}, d_{\mathcal{D}})$ .*

This is a straightforward exercise in topology and measure theory, starting by expressing the conditions on  $N$  of Definition 2.13 in terms of the càdlàg function  $g = \xi(N)$ .

Adapting the definition of  $d_{\mathcal{D}}^A$  of Proposition 3, we equip  $\mathcal{D}_{\text{exc}} \setminus \{0\}$  with the metric  $d_{\mathcal{D}}^A(f, g) = d_{\mathcal{D}}(f, g) + |A(f)^{-1} - A(g)^{-1}|$ , where  $A$  is the amplitude

of  $g$  given by  $A(g) := \sup\{|g(t)|, t \geq 0\}$ . With this definition, the following result follows from [1, Theorems IV.8 and IV.10].

**PROPOSITION 6.** *The  $\text{Stable}(1 + \alpha)$  excursion measure  $\nu_{\text{stb}}$  defined in (4.8) is boundedly finite for  $(\mathcal{D}_{\text{exc}} \setminus \{0\}, d_{\mathcal{D}}^A)$ , and it satisfies the integrability condition  $\int (\text{len}(g) \wedge 1) d\nu_{\text{stb}}(g) < \infty$ .*

Finally, we turn to point measures of clades and bi-clades such as  $F^y(N)$  and  $F^{\geq y}(N)$ , as defined in Definition 4.7.

**LEMMA 7.** *There exists a metric  $d_{\mathcal{N}}^A$  on  $\mathcal{N}_{\text{fin}}^{\text{sp}}$  and a set  $\tilde{\mathcal{N}}^{\text{sp}} \subset \mathcal{N}^{\text{sp}}$  with the following properties.*

- (i)  $(\mathcal{N}_{\text{fin}}^{\text{sp}}, d_{\mathcal{N}}^A)$  is isometric to a Borel subset of a complete, separable metric space.
- (ii) The Borel  $\sigma$ -algebra generated by  $d_{\mathcal{N}}^A$  equals that generated by the evaluation maps on measurable subsets of  $[0, \infty) \times \mathcal{E}$ .
- (iii) For  $y \in \mathbb{R}$ , the maps  $F^y$ ,  $F_0^y$ ,  $F^{\leq y}$ ,  $F_0^{\leq y}$ ,  $F^{\geq y}$ , and  $F_0^{\geq y}$  are measurable maps from  $\tilde{\mathcal{N}}^{\text{sp}}$  to  $\mathcal{N}([0, \infty) \times \mathcal{N}_{\text{fin}}^{\text{sp}})$ , where the latter is the space of counting measures that are boundedly finite on  $[0, \infty) \times \mathcal{N}_{\text{fin}}^{\text{sp}}$ .
- (iv)  $\mathcal{N}_{\text{fin}}^{\text{sp}} \subset \tilde{\mathcal{N}}^{\text{sp}}$ , and the law of the  $\text{PRM}(\text{Leb} \otimes \nu)$  on  $[0, \infty) \times \mathcal{E}$  is supported on  $\tilde{\mathcal{N}}^{\text{sp}}$ .

**PROOF.** By Proposition 4 there is a complete, separable metric  $d_{\mathcal{N}}$  on  $\mathcal{N}([0, \infty) \times \mathcal{E})$  that generates the same  $\sigma$ -algebra as the evaluation maps. Following Proposition 3, we define a modified metric  $d_{\mathcal{N}}^A(N, M) := d_{\mathcal{N}}(N, M) + |\hat{A}(\xi(N))^{-1} - \hat{A}(\xi(M))^{-1}|$  on  $\mathcal{N}_{\text{fin}}^{\text{sp}}$ , where for  $g \neq 0$ ,  $\hat{A}(g) = A(g)$  denotes amplitude, and we set  $\hat{A}(0) := -1$ . Let  $\tilde{\mathcal{N}}^{\text{sp}} := \bigcap_{y \in \mathbb{R}} \mathcal{N}^y$  where

$$\mathcal{N}^y := \mathcal{N}_{\text{fin}}^{\text{sp}} \cup \left\{ N \in \mathcal{N}^{\text{sp}} : \ell_N^y(t) \text{ exists } \forall t > 0, \lim_{t \uparrow \infty} \ell_N^y(t) = \infty \right\}.$$

(i) Consider  $\mathcal{N}([0, \infty) \times \mathcal{E}) \times (\{-1\} \cup [0, \infty))$  under the sum of  $d_{\mathcal{N}}$  in the first coordinate plus the Euclidean metric in the second coordinate. This space is complete and separable. Moreover,  $(\mathcal{N}_{\text{fin}}^{\text{sp}}, d_{\mathcal{N}}^A)$  is isometric to a measurable subset of this space via the map  $N \mapsto (N, \hat{A}(\xi(N))^{-1})$ .

(ii) Since  $d_{\mathcal{N}}^A$  is stronger than  $d_{\mathcal{N}}$ , it follows that  $\Sigma(\mathcal{N}_{\text{fin}}^{\text{sp}})$  is contained in the Borel  $\sigma$ -algebra generated by  $d_{\mathcal{N}}^A$ . By separability of  $(\mathcal{N}_{\text{fin}}^{\text{sp}}, d_{\mathcal{N}}^A)$ , open sets under  $d_{\mathcal{N}}^A$  can be described as countable unions of sets of the form  $B_{\mathcal{N}}(N, r) \cap B^A(N, r)$ , where this denotes the intersection of a ball under  $d_{\mathcal{N}}$  with a ball under the pseudometric  $|\hat{A}(\xi(\cdot))^{-1} - \hat{A}(\xi(\cdot))^{-1}|$ . Thus, it suffices to confirm that  $B^A(N, r) \in \Sigma(\mathcal{N}_{\text{fin}}^{\text{sp}})$  for every  $N \in \mathcal{N}_{\text{fin}}^{\text{sp}}$  and  $r > 0$ . Indeed, balls

in the pseudometric  $|A(\cdot)^{-1} - A(\cdot)^{-1}|$  are open in the Skorokhod topology on  $\{g \in \mathcal{D}_{\text{stb}} : \text{len}(g) \in (0, \infty)\}$ . Finally, since Proposition 2.14 establishes that  $\xi: \mathcal{N}_{\text{fin}}^{\text{sp}} \setminus \{0\} \rightarrow \{g \in \mathcal{D}_{\text{stb}} : \text{len}(g) \in (0, \infty)\}$  is a measurable map, the  $B^A(N, r)$  are measurable.

(iii) Fix  $y \in \mathbb{R}$ ,  $N \in \mathcal{N}^y$ , and  $\epsilon > 0$ . By the right-continuity of  $\xi(N)$ , this process can only have finitely many excursions of amplitude at least  $\epsilon$  up to any inverse local time  $\tau_N^y(s)$ ,  $s \geq 0$ . Thus, the desired bounded finiteness follows from the property that sequences of bi-clades  $N_i$  with  $\lim_{i \uparrow \infty} A(\xi(N_i)) = 0$  cannot be bounded in  $d_N^A$ . As for measurability, this follows from the measurability of the local time process  $(\ell_N^y(t), t \geq 0)$ , Definition A.1 of  $V_0^y(N)$ , and the straightforward measurability of restriction maps on  $\mathcal{N}^{\text{sp}}$  and  $\mathcal{E}$ .

(iv) It is immediate from our definition of  $\tilde{\mathcal{N}}^{\text{sp}}$  that  $\mathcal{N}_{\text{fin}}^{\text{sp}} \subset \tilde{\mathcal{N}}^{\text{sp}}$ . The second claim, that the PRM law is supported on  $\tilde{\mathcal{N}}^{\text{sp}}$ , follows from Theorem 2.16 and [7, Lemma 20].  $\square$

**4. Skewer and cutoff functions.** In Proposition 3.5, we claim the measurability of the map  $\overline{\text{SKEWER}}$  from  $(\mathcal{N}_{\text{fin}}^{\text{sp},*}, \Sigma(\mathcal{N}_{\text{fin}}^{\text{sp},*}))$  to  $\mathcal{C}([0, \infty), \mathcal{I})$  equipped with the Borel  $\sigma$ -algebra generated by uniform convergence.

LEMMA 8. *The map  $N \mapsto \text{SKEWER}(y, N)$  is measurable on the set  $\mathcal{N}_{\text{fin}}^{\text{sp},\circ}$  of point processes of spindles  $N \in \mathcal{N}_{\text{fin}}^{\text{sp}}$  that satisfy conditions (i) and (ii) of Definition 3.4 of  $\mathcal{N}_{\text{fin}}^{\text{sp},*}$ .*

PROOF. We have established in Proposition 2.20 that  $N \mapsto \xi(N)$  is a measurable map from  $(\mathcal{N}^{\text{sp}}, \Sigma(\mathcal{N}^{\text{sp}}))$  to  $(\mathcal{D}_{\text{stb}}, \Sigma(\mathcal{D}_{\text{stb}}))$ . By Definition 3.1 of the aggregate mass process, we deduce the measurability of the map  $N \mapsto M_{N, \xi(N)}^y(t)$  from  $\mathcal{N}_{\text{fin}}^{\text{sp}}$  to  $[0, \infty]$ , for  $(y, t)$  fixed. Let  $\mathcal{D}^*$  denote the set of non-decreasing càdlàg functions that are supported on intervals  $[0, L]$ ,  $L \in [0, \infty)$  and whose closed ranges have zero Lebesgue measure. Since  $M_{N, \xi(N)}^y(t)$  is non-decreasing in  $t$ , we conclude that for fixed  $y$  the map  $N \mapsto (M_{N, \xi(N)}^y(t), t \in [0, \text{len}(N)])$  is measurable from  $\mathcal{N}_{\text{fin}}^{\text{sp}}$  to  $\mathcal{D}^*$ .

Consider the map  $G$  that takes  $\beta \in \mathcal{I}_H$  to the closed, bounded, Lebesgue-null set  $G(\beta) = [0, \|\beta\|] \setminus \bigcup_{U \in \beta} U$ . The map  $g \mapsto G^{-1}(\text{range}(g))$  is continuous from the Skorokhod topology on  $\mathcal{D}^*$  to the Hausdorff topology on  $\mathcal{I}_H$ . Thus,  $N \mapsto \text{SKEWER}(y, N)$  is measurable from  $\mathcal{N}_{\text{fin}}^{\text{sp},\circ}$  to  $(\mathcal{I}_H, d_H)$  for fixed  $y$ . From [8, Theorem 2.3(c)], the Borel  $\sigma$ -algebra generated by  $d_{\mathcal{I}}$  on  $\mathcal{I}$  equals that generated by the Hausdorff metric,  $d_H$ . Thus, the map  $N \mapsto \text{SKEWER}(y, N)$  is measurable from  $\mathcal{N}_{\text{fin}}^{\text{sp},\circ}$  to  $(\mathcal{I}, d_{\mathcal{I}})$  for  $y$  fixed.  $\square$

PROOF OF PROPOSITION 3.5. By Theorem 2.3,  $(\mathcal{I}, d_{\mathcal{I}})$  is separable. From

this it follows that the  $\sigma$ -algebra on  $\mathcal{C}([0, \infty), \mathcal{I})$  generated by uniform convergence equals that generated by the evaluation maps [2, Theorem 14.5]. Hence, Proposition 3.5 is a consequence of Lemma 8.  $\square$

Lemma 4.8 includes the measurability of the functions  $\text{CUTOFF}^{\leq}(y, N)$  and  $\text{CUTOFF}^{\geq}(y, N)$ , as functions of  $F_0^{\leq y}(N)$  and  $F_0^{\geq y}(N)$ , and that the level filtration  $\mathcal{F}^y$  on  $\mathcal{N}^{\text{sp}}$ , of Definition 4.6(i) is, up to PRM-null sets, generated by the anti-clade counting measure  $F_0^{\leq y}$  defined in Definition 4.7.

PROOF OF MEASURABILITY CLAIMS OF LEMMA 4.8. We establish measurability by expressing the concatenation formulas in terms of integrals. For convenience, we write  $F_{0,N}^{\leq y} := F_0^{\leq y}(N)$ . Setting

$$\begin{aligned} \tau_N^{\leq y}(s-) &:= \int_{[0,s) \times \mathcal{N}^{\text{sp}}} \text{len}(N') dF_{0,N}^{\leq y}(r, N'), \\ \text{CUTOFF}^{\leq}(y, N) &= \int \int \delta\left(\tau_N^{\leq y}(s-) + t, f\right) dN'(t, f) dF_{0,N}^{\leq y}(s, N'), \end{aligned}$$

and correspondingly for  $\text{CUTOFF}^{\geq}(y, N)$ . Finally,  $F_0^{\leq y}$  generates  $\mathcal{F}^y$  up to events on which level  $y$  is not nice for  $N$ , which by Proposition A.3 are null for the PRM.  $\square$

In Proposition 5.3(iv) we claim that  $F_0^{\geq 0}$  is measurable on the (measurable) set  $\mathcal{S}$  of point measures where  $\text{SKEWER}(0, N) \in \mathcal{I}$ , and that  $\beta \mapsto \mathbf{P}_\beta^{(\alpha)}(F_0^{\geq 0} \in \cdot)$  is a stochastic kernel.

PROOF OF PROPOSITION 5.3(iv). First,  $\text{SKEWER}(0, \mathbf{N}_\beta) = \beta$  for every  $\beta \in \mathcal{I}$ , so the laws  $\mathbf{P}_\beta^{(\alpha)}$  are supported on  $\mathcal{S}$ . Now, we need only construct the desired measurable map  $\phi$ , as the stochastic kernel claim follows from this and Proposition 5.3(ii). We present  $\phi(N)$  in the case  $N = \mathbf{N}_\beta$ , but this construction applies to any  $N \in \mathcal{S}$ . Define

$$\mathbf{G}_1 := \sum_{[a,b] \in V_0^0(\mathbf{N}_\beta)} \delta\left(a, \mathbf{N}_\beta|_{[a,b]}^{\leftarrow}, m^0\left(\mathbf{N}_\beta|_{[a,b]}^{\leftarrow}\right)\right).$$

Then for each  $U \in \beta$  we get  $\mathbf{N}_U = \mathbf{N}_\beta|_{[a,b]}^{\leftarrow}$  for some  $[a, b] \in V_0^0(\mathbf{N}_\beta)$ , and

$$\mathcal{D}_\beta(U) = \Gamma(1 - \alpha/q) \lim_{h \downarrow 0} h^{\alpha/q} \mathbf{G}_1([0, a) \times \mathcal{N}_{\pm \text{cld}}^{\text{sp}} \times (h, \infty)) =: D_{[a,b]}.$$

Finally,  $F_0^{\geq 0}(\mathbf{N}_\beta) = \phi(\mathbf{N}_\beta) := \sum_{[a,b] \in V_0^0(\mathbf{N}_\beta)} \delta(D_{[a,b]}, \mathbf{N}_\beta|_{[a,b]}^{\leftarrow})$ . The measurability of the preceding transformations follows from the measurability of restriction maps and the existence of measurable enumerations of points of a point process, per [6, Proposition 9.1.XII].  $\square$

Lemma 5.4 collects several statements relating the skewer process to cutoff processes and point processes of clades.

PROOF OF LEMMA 5.4. (i). This follows from the definitions in (4.16). See Figure 4.2.

Before proceeding to prove (ii) we note that, in the general setting of (i), we make no claim in the case  $y = z$ . These formulas fail in cases where  $y = z$  and this is a level at which a spindle of  $N$  is born or dies discontinuously. For example, if a spindle  $f_t$  of  $N$  dies discontinuously at level  $z$ , then there is no broken spindle  $\hat{f}_t^z$  incorporated into  $\text{CUTOFF}^{\geq}(z, N)$ . Thus, while  $\text{SKEWER}(z, N)$  has a block of size  $f_t((z - \xi_N(t-)) -)$  corresponding to this spindle,  $\text{SKEWER}(0, \text{CUTOFF}^{\geq}(z, N), \text{CUTOFF}^{\geq}(z, \xi(N)))$  has no such block.

Also, we claim that for  $\mathbf{N}$  a  $\text{PRM}(\text{Leb} \otimes \nu_{\text{BESQ}}^{(-2\alpha)})$ , it is a.s. the case that for every  $t \geq 0$ ,

$$\text{SKEWER}\left(y, \mathbf{N}|_{[0,t]}\right) = \begin{cases} \text{SKEWER}\left(y, \text{CUTOFF}^{\leq}(z, \mathbf{N}|_{[0,t]})\right) & \text{if } y \leq z, \\ \text{SKEWER}\left(y - z, \text{CUTOFF}^{\geq}(z, \mathbf{N}|_{[0,t]})\right) & \text{if } y \geq z. \end{cases}$$

The same holds for  $\mathbf{N}_\beta$ , for any  $\beta \in \mathcal{I}_H$ , with  $z > 0$ .

To show this, the argument in the proof of Proposition 5.3(iii) also shows that

$$\begin{aligned} \xi(\text{CUTOFF}^{\leq}(z, \mathbf{N}|_{[0,t]})) &= \text{CUTOFF}^{\leq}(z, \xi(\mathbf{N})|_{[0,t]}) \\ \xi(\text{CUTOFF}^{\leq}(z, \mathbf{N}_\beta|_{[0,t]})) &= \text{CUTOFF}^{\leq}(z, \xi(\mathbf{N}_\beta)|_{[0,t]}), \end{aligned}$$

and likewise for  $\text{CUTOFF}^{\geq}(z, \cdot)$ . In particular, that argument uses the a.s. summability of lifetimes of leftmost spindles  $\zeta(\mathbf{f}_U)$  to show that the concatenation of the scaffoldings of clades  $\star_U \xi(\mathbf{N}_U)$  equals the scaffolding of their concatenation  $\xi(\star_U \mathbf{N}_U)$ . The same argument applies here.

Next, since no spindles in  $\mathbf{N}$  or  $\mathbf{N}_\beta$  are born or die discontinuously at any level above 0, every spindle  $f_t$  of  $\mathbf{N}$  or  $\mathbf{N}_\beta$  that is alive at level  $z > 0$  has non-trivial broken components  $\hat{f}_t^z$  and  $\check{f}_t^z$  about level  $z$ . Thus, the statement of (i) still holds a.s. for  $\mathbf{N}_\beta$  if we replace strict inequalities on the conditions for the two expressions by weak inequalities.

(ii). This follows from assertion (i) via Lemma 4.8, which relates the cutoff function  $\text{CUTOFF}^{\geq}(y, \cdot)$  to  $F_0^{\geq y}$ , and via the observation that the skewer map commutes with concatenation of bi-clades.

(iii). Definition 5.2 of  $F_0^{\geq 0}(\mathbf{N}_\beta)$  has the property that, if  $\beta$  is nice in the sense described in the assertion, then  $F_0^{\geq 0}(\mathbf{N}_\beta)$  does not have two points coinciding at the same time. Thus, the conclusion of Lemma 4.8 applies to

it, and  $\text{CUTOFF}^{\geq}(0, \mathbf{N}_\beta)$ , which equals  $\mathbf{N}_\beta$ , may be recovered from  $F_0^{\geq 0}(\mathbf{N}_\beta)$ . Thus, the claim follows by the same argument as when proving the claim established in the proof of (i) above.

(iv). This follows from the last assertion of Lemma 4.8.  $\square$

## REFERENCES

- [1] Jean Bertoin. *Lévy processes*, volume 121 of *Cambridge Tracts in Mathematics*. Cambridge University Press, Cambridge, 1996.
- [2] Patrick Billingsley. *Convergence of probability measures*. Wiley Series in Probability and Statistics: Probability and Statistics. John Wiley & Sons, Inc., New York, second edition, 1999. A Wiley-Interscience Publication.
- [3] J. T. Chang and D. Pollard. Conditioning as disintegration. *Statist. Neerlandica*, 51(3):287–317, 1997.
- [4] L. Chaumont. Excursion normalisée, méandre et pont pour les processus de Lévy stables. *Bull. Sci. Math.*, 121(5):377–403, 1997.
- [5] D. J. Daley and D. Vere-Jones. *An introduction to the theory of point processes. Vol. I. Probability and its Applications* (New York). Springer-Verlag, New York, second edition, 2003. Elementary theory and methods.
- [6] D. J. Daley and D. Vere-Jones. *An introduction to the theory of point processes. Vol. II. Probability and its Applications* (New York). Springer, New York, second edition, 2008. General theory and structure.
- [7] Noah Forman, Soumik Pal, Douglas Rizzolo, and Matthias Winkel. Uniform control of local times of spectrally positive stable processes. *Ann. Appl. Probab.*, 28(4):2592–2634, 2018.
- [8] Noah Forman, Soumik Pal, Douglas Rizzolo, and Matthias Winkel. Metrics on sets of interval partitions with diversity. arXiv: 1907.02132 [math.PR], 2019.
- [9] Olav Kallenberg. *Foundations of modern probability*. Probability and its Applications (New York). Springer-Verlag, New York, second edition, 2002.
- [10] Daniel Revuz and Marc Yor. *Continuous martingales and Brownian motion*, volume 293 of *Grundlehren der Mathematischen Wissenschaften [Fundamental Principles of Mathematical Sciences]*. Springer-Verlag, Berlin, third edition, 1999.

DEPARTMENT OF MATHEMATICS & STATISTICS  
MCMMASTER UNIVERSITY  
1280 MAIN STREET WEST  
HAMILTON, ONTARIO L8S 4K1  
CANADA  
E-MAIL: [noah.forman@gmail.com](mailto:noah.forman@gmail.com)

DEPARTMENT OF MATHEMATICAL SCIENCES  
UNIVERSITY OF DELAWARE  
NEWARK DE 19716  
USA  
E-MAIL: [drizzolo@udel.edu](mailto:drizzolo@udel.edu)

DEPARTMENT OF MATHEMATICS  
UNIVERSITY OF WASHINGTON  
SEATTLE WA 98195  
USA  
E-MAIL: [soumikpal@gmail.com](mailto:soumikpal@gmail.com)

DEPARTMENT OF STATISTICS  
UNIVERSITY OF OXFORD  
24–29 ST GILES’  
OXFORD OX1 3LB  
UK  
E-MAIL: [winkel@stats.ox.ac.uk](mailto:winkel@stats.ox.ac.uk)
